# Supplementary material for: Offline Policy Evaluation and Optimization under Confounding
Source: arXiv:2211.16583 source file (2023-11-07)
Supplement: Supplementary file 1 [file clusterMDP.tex]

Through the recent work of \citet{ambuj2022mixmdp}, with enough data under Assumptions \ref{assump:global_u}, \ref{assump:mixing}, and \ref{assump:model_sep}, it is possible to infer the unobserved global confounder $u_n$ in each trajectory up to permutation, thereby distinguishing trajectories generated by different $u\sim P(u)$. 

% yw / first time use of u_n, maybe it is worth saying it is the confounder value of the n-th trajectory?

\begin{assumption}[Mixing]\label{assump:mixing}
The $U$ Markov chains on $\mathcal{S} \times \mathcal{A}$ induced by the various behavior policies $\pi(a \mid s, u)$, each achieve mixing to a stationary distribution $d_{u}(s,a)$ with mixing time $t_{mix, u}$. Define the overall mixing time of the mixture of MDPs to be $t_{mix} := \max_u t_{mix, u}$.
\end{assumption}

\begin{assumption}[Model Separation]\label{assump:model_sep}
There exist $\alpha, \Delta > 0$ so that for each pair $u_1, u_2$ of confounders, there exists a state action pair $(s,a)$ (possibly depending on $u_1, u_2$) so that the stationary distributions under each confounder $d_{u_1}(s,a), d_{u_2}(s,a) \geq \alpha$ and $\|\prob^{(u_1)}(\cdot \mid s,a) - \prob^{(u_2)}(\cdot \mid s,a)\|_2 \geq \Delta$.
\end{assumption}

As the paper mentions, Assumption~\ref{assump:model_sep} is merely saying that for any pair of labels, at least one visible state action pair witnesses a model difference $\Delta$. They call it the separating state-action pair. 

Additionally, Assumption~\ref{assump:mixing} is not a strong assumption, since any irreducible aperiodic finite state space Markov chain mixes to a unique stationary distribution. If the Markov chain is not irreducible, it mixes to a unique distribution determined by the irreducible component of the starting distribution.

The only requirement is thus aperiodicity, which is also technically superficial, as we now clarify. If the induced Markov chains were periodic with period $L$, we would have a finite set of stationary distributions $d_{u, l}(s,a)$ that the chain would cycle through over a single period, indexed by $l = 1 \to L$. One can follow the proofs to verify that the guarantees continue to hold if we modify $\alpha$ in Assumption~\ref{assump:model_sep} to be a lower bound for $\min_{i,l} d_{u_i, l}(s,a)$ instead of just $\min_i d_{u_i}(s,a)$. With this modification, Assumption~\ref{assump:mixing} is not an assumption at all -- it is merely giving a name to the mixing times.

\subsection{Exact Clustering of Trajectories}

At the start of each trajectory, by \ref{assump:global_u} a different confounder $u \sim P(U)$ is drawn, corresponding to different models $\prob^{(u)}(\cdot|s,a):=\prob(\cdot|s,a,u)$ and policies $\pi_u(a|s) := \pi(a|s,u)$. We, therefore, satisfy the assumptions of \citet{ambuj2022mixmdp}, and so can leverage their method that achieves exact clustering while only explicitly requiring the number of trajectories $N_{traj}$ to be linear in $S$ and the trajectory length to be linear in the mixing time $t_{mix}$.

\begin{thm}[Exact Clustering Guarantee (Informal) from \cite{ambuj2022mixmdp}]\label{thm:clustering-informal}
With high probability, we can exactly recover all confounder labels (up to permutation) with $U^2S$ trajectories of length $U^{3/2} t_{mix}$, up to behavior-policy-and-model-specific constants $\alpha$ and $\Delta$ not explicitly dependent on $S, A$ or $U$.
\end{thm}

% yw / above, what is the U here? is it the cardinality of values U can take? (note above U is used in u~P(U))

\subsection{Clustering-Based OPE}

We use Algorithm~\ref{algo:clusterOPE} as a broad meta-algorithm that clusters the data and uses any OPE method on each cluster to obtain a final policy value estimate $\hat{V}_1(s_0 ; \pi_e)$. If the off-policy value estimator has a sample complexity $N_2(\delta, \epsilon, b)$ under some assumption $A(b)$ parameterized by a vector $b$, then we have the following sample complexity guarantee.

\begin{thm} \label{lemma:consistentClusters}
There are constants $H_0$, $N_0$ depending polynomially on $\alpha, \Delta, \min_u P(u)$ so that for $n$ trajectories of length $H \leq H_0t_{mix}\log(n)$, if

$$n \geq \max\left(U^2SN_0\log(3/\delta), \frac{2\log(3/\delta)}{\min(\epsilon^2, \min_u P(u)^2)}, N_2\left(\frac{\delta}{3}, \frac{\epsilon}{2}, b\right)\right)$$

then $|\hat{V}_1(s_0 ; \pi_e) - V_1(s_0 ; \pi_e)| < \epsilon$
\end{thm}

The first term in the maximization comes from the sample complexity for exact clustering, the second is needed for estimating the weights of confounders accurately and the third is the sample complexity of the OPE estimator. Usually, the assumption $A(b)$ needed by the OPE estimator is a concentrability assumption. We can instantiate $N_2(\delta, \epsilon, b)$ using Theorem 3.8 of \citet{yin2020asymptotically}, Corollary 1 of \citet{duan2020minimax}, or other off policy estimators listed in section 2 of \citet{zhang2022opelist} viewed in a tabular setting.

%IF H NOT GOING TO INFINITY, PROVIDE A NEW PAC BOUND ON VALUE ESTIMATION: DIFFERENT FROM SIMULATION LEMMA, NO NEED TO OBSERVE ALL STATES AND ACTIONS, JUST SEPARATING ONES

%OVERLAP WITH TARGET AND BEHAVIOR POLICY RESOLVED WITH DR PROPERTY -- ARE WE HIDING AN OVERLAP ASSUMPTION
%If data was collected from target policy instead of behavior policy, would we have estimated different models? Yes, if target policy has no model separation assumption. 
%But with DR properties on overlap and consistency results, this is mitigated.
%We are able to get these results because of the DR properties and consistency properties of the off-the-shelf estimator, allowing us to have model estimation error but recover a consistent OPE estimate

Therefore, under Assumptions \ref{assump:global_u}, \ref{assump:model_sep}, and \ref{assump:mixing}, we can provide a point estimate of the policy's value that is consistent.

\begin{algorithm}[h]
	\centering
	\caption{Clustering-Based OPE}
	\begin{algorithmic}[1]
		\STATE \textbf{input: } Number of clusters $U$, evaluation policy $\pi_e$.
		\STATE \textbf{run subroutine: } Perform clustering on trajectories, obtain clusters $C_1,...,C_U$.
		\STATE  Obtain cluster weight estimates $\hat{P}(u) := \frac{|C_u|}{N_{traj}}$.
        \STATE \textbf{run subroutine: } Estimate $\hat{V}_1(s_0; C_u, \pi_e)$ for each cluster $C_u$ via e.g. doubly robust estimators.
		\STATE \textbf{return: } Output the final policy value estimate $\hat{V}_1(s_0 ; \pi_e) = \sum_{u=1}^U \hat{P}(u_i) \hat{V}_1(s_0; C_u, \pi_e)$.
	\end{algorithmic}
\label{algo:clusterOPE}
\end{algorithm}
